# Supplementary material for: Confinement-Driven Acceleration of First-Passage Rates
Source: arXiv:2501.08571 source file (2025-01-15)
Supplement: Supplementary file 1 [file SM.pdf]

# Supplemental Material: Confinement-Driven Acceleration of First-Passage Rates

Won Kyu Kim[1,2,*]
[1]School of Computational Sciences, Korea Institute for Advanced Study, Seoul 02455, Korea
[2]Department of Physics and Astronomy, Seoul National University, Seoul 08826, Korea
(Dated: January 15, 2025)

## I. FICK-JACOBS APPROXIMATION

For two-dimesional (2D) systems, the Fick-Jacobs (FJ) approximation introduces the 1D entropic free energy landscape $U(x) = -k_B T \ln[w(x)/L]$ [1] and diffusivity $D(x) \approx D/[1 + (\mathrm{d}w(x)/\mathrm{d}x)^2/4]^{1/3}$ [2], where $w(x)$ is the length of position-dependent accessible cross-section and $L$ is the reference (system) length. The mean first-passage time [3] starting from the reflecting boundary at $x = 0$ and ending at the absorbing boundary at $x = L$ then leads to

$$\begin{aligned} \tau &= \int_0^L \mathrm{d}x \frac{\mathrm{e}^{\beta U(x)}}{D(x)} \int_0^x \mathrm{d}x' \mathrm{e}^{-\beta U(x')} \\ &\approx \frac{1}{D} \int_0^L \mathrm{d}x \left[ 1 + \frac{1}{4} \left( \frac{\mathrm{d}w(x)}{\mathrm{d}x} \right)^2 \right]^{1/3} \frac{1}{w(x)} \int_0^x \mathrm{d}x' w(x'). \end{aligned} \tag{S1}$$

For the tunnel confinement shown in Fig. 1 in the main text, the cross-section length in the tunnel is $w(x) = L\mathrm{e}^{-\beta U_B}$, while $w(x) = L$ outside the tunnel. Hence, we consider an energy barrier $U(x)$:

$$U(x) = \begin{cases} U_B, & \text{if } 0 < x \le x_B. \\ U_B \frac{x_B + \delta - x}{\delta}, & \text{if } x_B < x \le x_B + \delta. \\ 0, & \text{otherwise,} \end{cases} \tag{S2}$$

as depicted in Fig. S1.

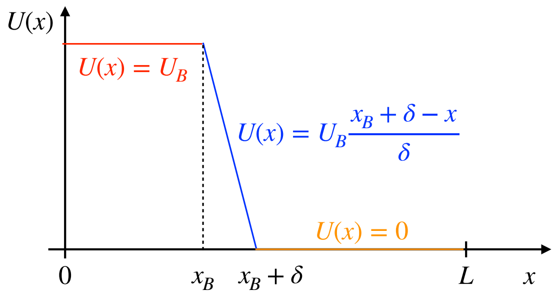


FIG. S1: One-dimensional energy barrier $U(x)$, consisting of a linear segment between two flat energy levels, $U_B$ and 0.

*Electronic address: wonkyukim@snu.ac.kr

We decompose the integral as follows:

$$\begin{aligned}
\tau D &= \left\{\int_0^{x_B} + \int_{x_B}^{x_B+\delta} + \int_{x_B+\delta}^{L}\right\} \mathrm{d}x\ \mathrm{e}^{\beta U(x)} \int_0^x \mathrm{d}x' \mathrm{e}^{-\beta U(x')}. \\
&= \int_0^{x_B} \mathrm{d}x\ \mathrm{e}^{\beta U_B} \int_0^x \mathrm{d}x' \mathrm{e}^{-\beta U_B} \\
&+ \int_{x_B}^{x_B+\delta} \mathrm{d}x\ \left[1+\frac{1}{4}\left(\frac{\mathrm{d}w(x)}{\mathrm{d}x}\right)^2\right]^{1/3} \mathrm{e}^{\beta U_B \frac{x_B+\delta-x}{\delta}} \left\{\int_0^{x_B} \mathrm{d}x' \mathrm{e}^{-\beta U_B} + \int_{x_B}^{x} \mathrm{d}x' \mathrm{e}^{-\beta U_B \frac{x_B+\delta-x'}{\delta}}\right\} \\
&+ \int_{x_B+\delta}^{L} \mathrm{d}x\ \mathrm{e}^0 \left\{\int_0^{x_B} \mathrm{d}x' \mathrm{e}^{-\beta U_B \frac{x'}{x_B}} + \int_{x_B}^{x_B+\delta} \mathrm{d}x' \mathrm{e}^{-\beta U_B \frac{x_B+\delta-x'}{\delta}} + \int_{x_B+\delta}^{x} \mathrm{d}x' \mathrm{e}^0\right\},
\end{aligned} \tag{S3}$$

which yields the mean first-passage rate (MFPR) in the limit $\delta \to 0$, $k/k_0 = L^2/(2D\tau)$,

$$\frac{k}{k_0} = \frac{1}{2(x_B/L)^2 - 2x_B/L + 1 + 2\mathrm{e}^{-\beta U_B}(1-x_B/L)x_B/L}. \tag{S4}$$

## II. 2D SIMULATION FOR A TUNNEL

We use the LAMMPS software [4] to perform Brownian dynamics (BD) simulations in the canonical ($NVT$) ensemble. Figure S2 shows the simulation setup, where a tunnel of width $w = L\mathrm{e}^{-\beta U_B}$ is extended along the $x$ direction. The blue particles depict the boundary, including the tunnel, and are composed of immobile hard-sphere particles overlapped with interparticle distance of $0.5\sigma$. The box size is $2L \times L$, where $L = 20\sigma$ is the box length in the $y$ direction, and $\sigma$ is the particle diameter. The simulation box is symmetric around the center, which is equivalent to imposing a reflecting boundary at $x = 0$.

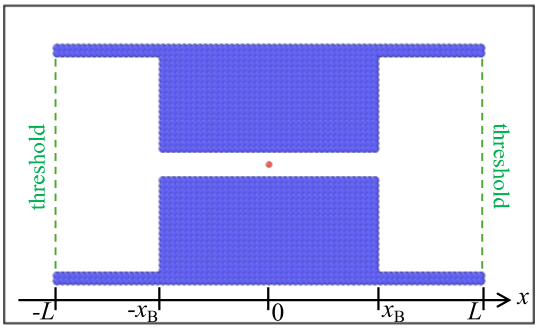


FIG. S2: Simulation of a tunnel with width $w = L\mathrm{e}^{-\beta U_B}$, extended along the $x$ direction and with mirror symmetry around $x = 0$. Here, $\beta U_B = 2.2$ and $x_B = 0.5L$.

A Brownian particle, identical to the obstacle particles but mobile, starts at the center of the box, and the first-passage time is recorded upon reaching $x = \pm L$ for the first time. For interactions between all particles, we use the Weeks–Chandler–Andersen (WCA) potential [5], a Lennard–Jones potential truncated at its minimum and shifted to zero:

$$U_{WCA}(r) = 4\epsilon\left[\left(\frac{\sigma}{r}\right)^{12} - \left(\frac{\sigma}{r}\right)^{6}\right] + \epsilon \quad \text{if } r < r_c = 2^{1/6}\sigma, \quad \text{otherwise zero,} \tag{S5}$$

with interaction strength $\epsilon = 1\ k_BT$, width $\sigma$, and cutoff $r_c = 2^{1/6}\sigma$.

The iteration time step is $\delta\tau = 0.001\tau$. The average time required for diffusion over the distance $L$ is $t = L^2/(2D) = 200\ \tau$, corresponding to $2 \times 10^5$ time steps. For each parameter set, we collect 2000 first-passage times, resulting in a total simulation time of about $10^8$ steps per parameter set.

## III. 2D SIMULATION FOR POSITION-DEPENDENT TUNNEL

For the 2D simulation with position-dependent tunnel [Fig. 2(b) in the main text], we also perform BD simulations with obstacle hard particles. A box has a side length $L = 50\sigma$ (unit length), and the particle diameter is set to $\sigma$ [see Fig. 2(b) in the main text].

The same WCA hard-particle interactions between all particles and reflecting boundaries at $x = -\sigma$, $y = -\sigma$, and $y = L + \sigma$ are considered.

The iteration time step is $\delta\tau = 0.0005\tau$, where the time unit is defined as $\tau = \sqrt{mL^2/k_BT}$. Here, $m$ represents the unit mass, and $k_BT = 1/\beta$ is the thermal energy. The average time required for diffusion over the distance is estimated as $10^5$ time steps. For each parameter set, we collect approximately $10^3$ first-passage events, resulting in a total simulation time of about $10^8$ steps per parameter set.

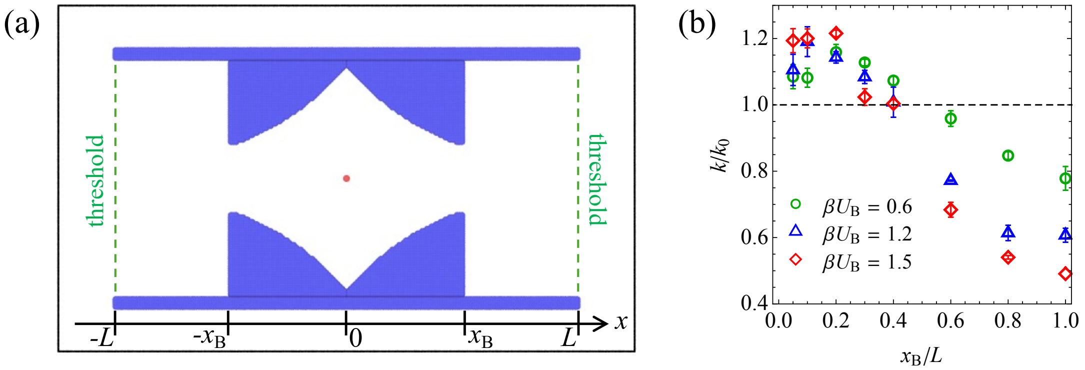


FIG. S3: (a) Simulation extended along the $x$ direction with mirror symmetry around $x = 0$. Here, $\beta U_B = 1.2$ and $x_B = 0.5L$. (b) Mean first-passage rate $k(x_B)/k_0$ for different $U_B$.

## IV. EXTENDED 2D SIMULATION WITH MIRROR SYMMETRY

In addition to the 2D confinement simulations with the reflecting wall at $x = 0$ considered in the main text, we also perform simulations with mirror symmetry around $x = 0$, which is extended along the $x$ direction, as shown in Fig. S3(a). The mean first-passage rates $k(x_B, U_B)/k_0$ from these simulations are shown in Fig. S3(b), exhibiting nonmonotonic behavior consistent with the results presented in the main text.

## V. DERIVATION OF EQ. (1)

Consider an energy barrier $U(x)$ as depicted in Fig. S4:

$$U(x) = \begin{cases} U_B \frac{x}{x_B}, & \text{if } 0 < x \le x_B. \\ U_B \frac{x_B+\delta-x}{\delta}, & \text{if } x_B < x \le x_B+\delta. \\ 0, & \text{otherwise.} \end{cases} \tag{S6}$$

With this piecewise potential $U(x)$, the mean first-passage time [3] can be calculated for a particle starting at the reflecting boundary at $x = 0$ and ending at the absorbing boundary at $x = L$:

$$\tau = \int_0^L \mathrm{d}x \frac{\mathrm{e}^{\beta U(x)}}{D} \int_0^x \mathrm{d}x' \mathrm{e}^{-\beta U(x')}. \tag{S7}$$

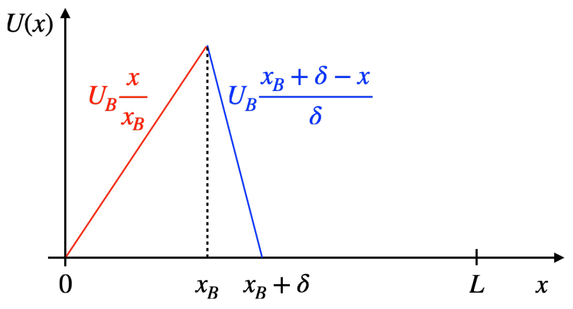


FIG. S4: One-dimensional energy barrier $U(x)$, consisting of two linear segments and a flat energy level.

Assuming $D$ is constant, we decompose the integral for $\tau$ as follows:

$$\begin{aligned}
\tau D &= \left\{\int_0^{x_B} + \int_{x_B}^{x_B+\delta} + \int_{x_B+\delta}^{L}\right\} \mathrm{d}x\, \mathrm{e}^{\beta U(x)} \int_0^x \mathrm{d}x' \mathrm{e}^{-\beta U(x')}. \\
&= \int_0^{x_B} \mathrm{d}x\, \mathrm{e}^{\beta U_B \frac{x}{x_B}} \int_0^x \mathrm{d}x' \mathrm{e}^{-\beta U_B \frac{x'}{x_B}} \\
&\quad + \int_{x_B}^{x_B+\delta} \mathrm{d}x\, \mathrm{e}^{\beta U_B \frac{x_B+\delta-x}{\delta}} \left\{\int_0^{x_B} \mathrm{d}x' \mathrm{e}^{-\beta U_B \frac{x'}{x_B}} + \int_{x_B}^{x} \mathrm{d}x' \mathrm{e}^{-\beta U_B \frac{x_B+\delta-x'}{\delta}}\right\} \\
&\quad + \int_{x_B+\delta}^{L} \mathrm{d}x\, \mathrm{e}^{0} \left\{\int_0^{x_B} \mathrm{d}x' \mathrm{e}^{-\beta U_B \frac{x'}{x_B}} + \int_{x_B}^{x_B+\delta} \mathrm{d}x' \mathrm{e}^{-\beta U_B \frac{x_B+\delta-x'}{\delta}} + \int_{x_B+\delta}^{x} \mathrm{d}x' \mathrm{e}^{0}\right\}.
\end{aligned} \tag{S8}$$

This reveals that the rescaled mean first-passage time $\tau/(L^2/(2D))$ is a quadratic function of $x_B/L$:

$$2D\tau/L^2 = C_2 \left(\frac{x_B}{L}\right)^2 - C_1 \left(\frac{x_B}{L}\right) + C_0, \tag{S9}$$

where the coefficients are given by

$$C_2 = \frac{2\mathrm{e}^{-\beta U_B}\beta U_B + (\beta U_B - 4)\beta U_B + 2\mathrm{e}^{\beta U_B} - 2}{(\beta U_B)^2}, \tag{S10}$$

$$C_1 = \frac{-\mathrm{e}^{-\beta U_B}\left[2\delta\left(2\beta U_B + \mathrm{e}^{\beta U_B}\left((\beta U_B - 2)\beta U_B + \mathrm{e}^{\beta U_B} - 2\right) + 1\right) - 2L\left(\mathrm{e}^{\beta U_B}(\beta U_B - 1) + 1\right)\beta U_B\right]}{L(\beta U_B)^2}, \tag{S11}$$

$$C_0 = \frac{\mathrm{e}^{-\beta U_B}\left[2\delta(\delta\beta U_B + \delta - L\beta U_B) + \mathrm{e}^{\beta U_B}\left(-2\delta^2 + (\beta U_B)^2(\delta - L)^2 + 2\delta L\beta U_B\right)\right]}{L^2(\beta U_B)^2}. \tag{S12}$$

This result is exact, and Fig. S5 presents the mean first-passage rate $k/k_0 = L^2/(2D\tau)$ using Eq. (S9) as a function of $x_B$ for various values of $\beta U_B$ and a fixed $\delta = 0.1L$. The rate $k/k_0$ exhibits a highly nonmonotonic dependence on $x_B$ and $U_B$, reaching a maximum that can exceed unity.

Notably, Eq. (S9) remains finite in the limit $\delta \to 0$, that is, for the linear barrier case discussed in the main text. In this limit, the coefficients simplify to

$$C_2 = \frac{2\mathrm{e}^{-\beta U_B}\beta U_B + (\beta U_B - 4)\beta U_B + 2\mathrm{e}^{\beta U_B} - 2}{(\beta U_B)^2}, \tag{S13}$$

$$C_1 = \frac{2\left(\beta U_B - 1 + \mathrm{e}^{-\beta U_B}\right)}{\beta U_B}, \tag{S14}$$

$$C_0 = 1. \tag{S15}$$

Therefore, one finds

$$\begin{aligned}
k/k_0 &\equiv L^2/(2D\tau) \\
&= \frac{1/C_2}{\left(\frac{x_B}{L}\right)^2 - \frac{C_1}{C_2}\left(\frac{x_B}{L}\right) + \frac{1}{C_2}} \\
&= \frac{\mathcal{A}}{\left(\frac{x_B}{L} - \lambda^*\right)^2 + \mathcal{A} - {\lambda^*}^2},
\end{aligned} \tag{S16}$$

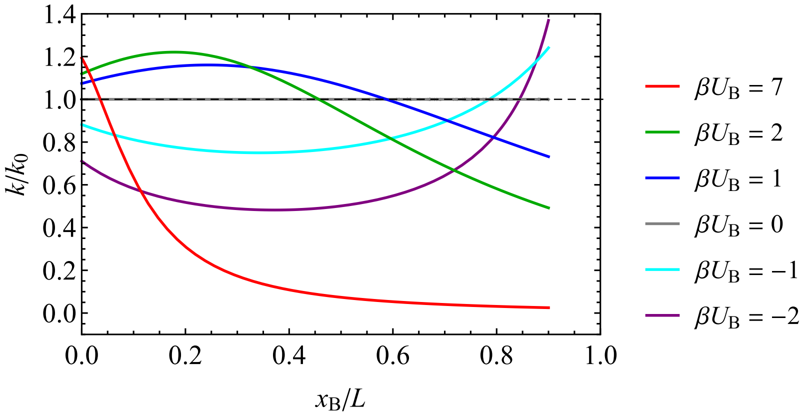


FIG. S5: The mean first-passage rate $L^2/(2D\tau)$, the inverse of Eq. (S9), as a function of $x_B$ for different values of $\beta U_B$ and the fixed value of $\delta = 0.1L$.

which is the main result given in Eq. (1), the Lorentzian-like function in the main text, where the location parameter $\lambda^*$ is

$$\lambda^* \;=\; \mathcal{A}(\mathcal{H}+1), \tag{S17}$$

with

$$\mathcal{A} \;=\; \frac{\beta U_B}{2\mathcal{H}(\beta U_B - \mathrm{e}^{\beta U_B}) + \beta U_B - 2},$$
$$\mathcal{H} \;=\; \frac{\mathrm{e}^{-\beta U_B} - 1}{\beta U_B}.$$

## VI. RESULTS WITH CORRECTION IN $D(x)$

The Fick–Jacobs approach includes a correction factor for $D(x) \approx D/[1 + (\mathrm{d}w(x)/\mathrm{d}x)^2/4]^{1/3}$ [1, 2]. Using $w(x) = L\mathrm{e}^{-\beta U(x)}$ with $U(x)$ given in Eq. (S6) and $D(x) = D/[1 + (\mathrm{d}w(x)/\mathrm{d}x)^2/4]^{1/3}$, we calculate the mean first-passage time given in Eq. (S7) consistently for $\delta \approx 0$ [see Fig. S6].

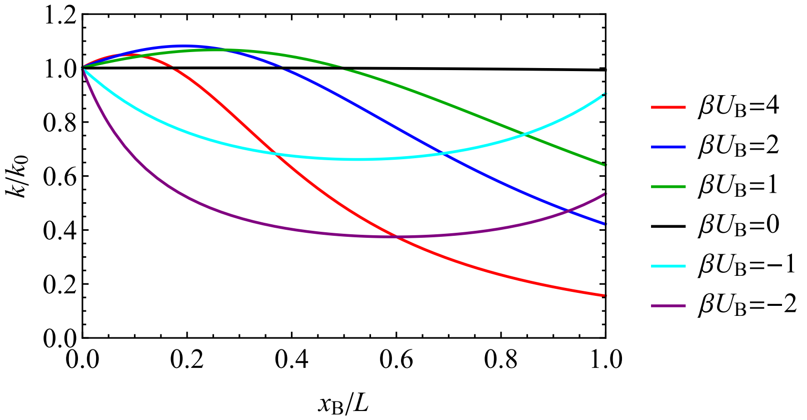


FIG. S6: The mean first-passage rate $L^2/(2D\tau)$ incorporating the position-dependent correction of $D(x)$, as a function of $x_B$ for different values of $\beta U_B$ and the fixed value of $\delta = 0.001L$.

## VII. LOCATION PARAMETER

The location parameter $\lambda^*$ as a function of $U_B$ given in Eq. (2) in the main text is shown in Fig. S7. First, the decaying $\lambda^*$ in the limit $U_B \to \infty$ signifies that the MFP rate $k$ tends to a decreasing monotonic function, in which the FP process is slower than the free diffusion.

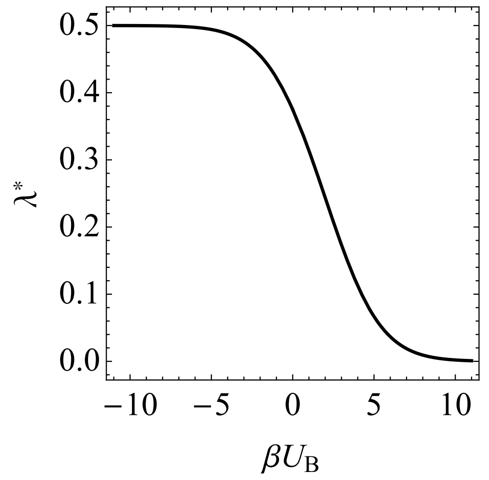


FIG. S7: Location parameter $\lambda^*$ given in Eq. (S17) versus the barrier height $\beta U_B$.

Interestingly, the location parameter approaches $\lambda^* = 1/2$ in the limit $U_B \to -\infty$, indicating that the trapping well [downhill in Fig. 2(a-ii)] with $x_B = 0.5L$ is the optimal confinement to trap a particle. Moreover, we find $\lambda^* = 3/8 \equiv \lambda_0^*$ at vanishing $U_B$. This means that in designing an optimal trap, $\lambda_0^*$ serves as an indicator of position of $x_B$ as an upper bound.

## VIII. 1D BROWNIAN DYNAMICS SIMULATION

We iteratively solve the equation $\tilde{x}(\tilde{t}+\delta\tilde{t}) = \tilde{x}(\tilde{t}) - \mathrm{d}(\beta U)/\mathrm{d}\tilde{x}\delta\tilde{t} + \sqrt{2\delta\tilde{t}}, r(\tilde{t})$, where $\tilde{x} = x/L$ denotes the rescaled position, $\tilde{t} = tD/L^2$ is the rescaled time, and $r(\tilde{t})$ is a Gaussian random variable with zero mean and unit variance. We use a time step of $\delta\tau = 3 \times 10^{-5}\tau$ and collect five independent datasets, each containing approximately 2000 first-passage times across various values of $x_B$ and $U_B$.

In these simulations, $U(x)$ vanishes for $x_B < x < L$ and exhibits a discontinuous drop at $x = x_B$. To account for the barrier $U(x_B)$, a crossing event from $x(\tilde{t}) > x_B$ to $x(\tilde{t}+\delta\tilde{t}) \leq x_B$ is allowed with probability $\mathrm{e}^{-\beta U_B}$. If the crossing is not accepted, the particle remains at $x(\tilde{t}+\delta\tilde{t}) = x(\tilde{t})$. This method resembles the Metropolis–Hastings algorithm [6, 7], which has previously been employed to simulate particle binding in Markov processes [8]. Once the time step is sufficiently small ($\delta\tau \sim 10^{-5}\tau$), this method performs very well, as shown in Fig. 4 of the main text.

## IX. DERIVATION OF TRANSMISSION PROBABILITY, EQ. (3)

Consider the Smoluchowski equation of a probability density $p(x)$ in a steady state with a constant flux $j$:

$$j = -D(x)\left[\frac{\mathrm{d}p(x)}{\mathrm{d}x} + p(x)\frac{\mathrm{d}\beta U(x)}{\mathrm{d}x}\right], \tag{S18}$$

which yields the flux with the solution $p(x)$ and one boundary $x = L$,

$$j = \frac{p(x)\mathrm{e}^{\beta U(x)} - p(L)\mathrm{e}^{\beta U(L)}}{\int_x^L \mathrm{d}x'\mathrm{e}^{\beta U(x')}/D(x')}. \tag{S19}$$

By applying an absorbing boundary condition at $x = L$, i.e., $p(L) = 0$, one finds

$$p(x) = j\mathrm{e}^{-\beta U(x)}\int_x^L \mathrm{d}x'\frac{\mathrm{e}^{\beta U(x')}}{D(x')}. \tag{S20}$$

Using the normalization condition, $\int_0^L \mathrm{d}x\ p(x) = 1$, one finds

$$j = \frac{1}{\int_0^L \mathrm{d}x\ \mathrm{e}^{-\beta U(x)} \int_x^L \mathrm{d}x' \frac{\mathrm{e}^{\beta U(x')}}{D(x')}}. \tag{S21}$$

Therefore, the probability density is

$$p(x) = \frac{\mathrm{e}^{-\beta U(x)} \int_x^L \mathrm{d}x' \frac{\mathrm{e}^{\beta U(x')}}{D(x')}}{\int_0^L \mathrm{d}x\ \mathrm{e}^{-\beta U(x)} \int_x^L \mathrm{d}x' \frac{\mathrm{e}^{\beta U(x')}}{D(x')}}, \tag{S22}$$

which yields the probability for being in $x_B < x \leq L$ with a constant $D$:

$$\mathcal{P}_{\mathrm{trans}} = \frac{\int_{x_B}^L \mathrm{d}x\ \mathrm{e}^{-\beta U(x)} \int_x^L \mathrm{d}x' \mathrm{e}^{\beta U(x')}}{\int_0^L \mathrm{d}x\ \mathrm{e}^{-\beta U(x)} \int_x^L \mathrm{d}x' \mathrm{e}^{\beta U(x')}}. \tag{S23}$$

For $U(x)$ given in Eq. (S6) and following the approach shown in Eq. (S8) in the limit $\delta \to 0$, one can find

$$\mathcal{P}_{\mathrm{trans}} = \frac{k}{k_0}\left(1 - \frac{x_B}{L}\right)^2, \tag{S24}$$

as shown in Eq. (3) in the main text.

[1] R. Zwanzig, The Journal of Physical Chemistry **96**, 3926 (1992).
[2] D. Reguera and J. Rubi, Physical Review E **64**, 061106 (2001).
[3] W. K. Kim and R. R. Netz, The Journal of Chemical Physics **143**, 224108 (2015).
[4] S. Plimpton, Journal of Computational Physics **117**, 1 (1995).
[5] J. D. Weeks, D. Chandler, and H. C. Andersen, The Journal of Chemical Physics **54**, 5237 (1971).
[6] N. Metropolis, A. W. Rosenbluth, M. N. Rosenbluth, A. H. Teller, and E. Teller, The journal of chemical physics **21**, 1087 (1953).
[7] W. K. Hastings, Biometrika **57**, 97 (1970), ISSN 00063444, 14643510.
[8] X. Xu, W. K. Kim, and J. Dzubiella, Physical Review E **103**, 032502 (2021).
